# Supplementary material for: Room temperature magnetic vortices in the van der Waals magnet Fe$_5$GeTe$_2$
Source: arXiv:2507.03454 ancillary file (2025-07-04)
Supplement: Supplementary file 1 [file supplement.pdf]

# Supplemental Material
# Room temperature magnetic vortices in the 2D magnet $Fe_5GeTe_2$

Elias Sfeir,[1] Carolin Schrader,[1] Florentin Fabre,[1] Jules Courtin,[2]
Céline Vergnaud,[2] Alain Marty,[2] Matthieu Jamet,[2] Frédéric Bonell,[2]
Isabelle Robert-Philip,[1] Vincent Jacques,[1] and Aurore Finco[1,*]

[1]*Laboratoire Charles Coulomb, Université de Montpellier, CNRS, Montpellier, France*
[2]*Université Grenoble Alpes, CNRS, CEA, SPINTEC, 38054 Grenoble, France.*

## CONTENTS

I. Structural characterization of the sample 2

II. Calibration of the diamond probe 3

III. Stray field from the edge of a uniformly magnetized film 4

IV. Estimation of the error in the extraction of $M_s$ 6

V. Choice of $K_u$ in the micromagnetic simulations of the vortices 9

VI. Vortices in disks 10

References 11

* aurore.finco@umontpellier.fr

# I. STRUCTURAL CHARACTERIZATION OF THE SAMPLE

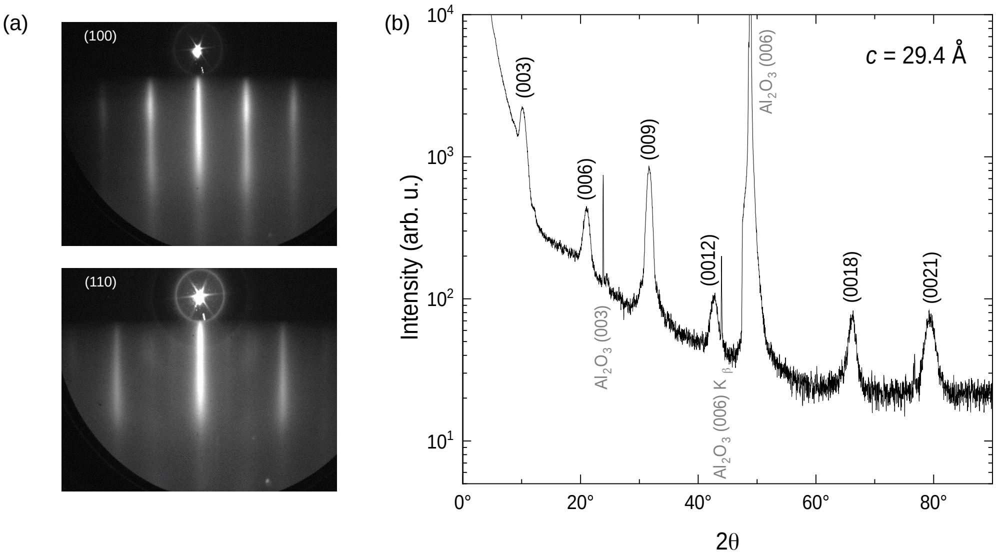


FIG. S1. (a) RHEED patterns, measured on the $Fe_5GeTe_2$ film before microstructuring, in the (100) and (110) reciprocal directions. (b) Out-of-plane $\theta/2\theta$ X-ray diffraction scan (Co source K$\alpha$= 1.79 Å). The measured $c$ lattice parameter is 29.4 Å (= 3 layers)

## II. CALIBRATION OF THE DIAMOND PROBE

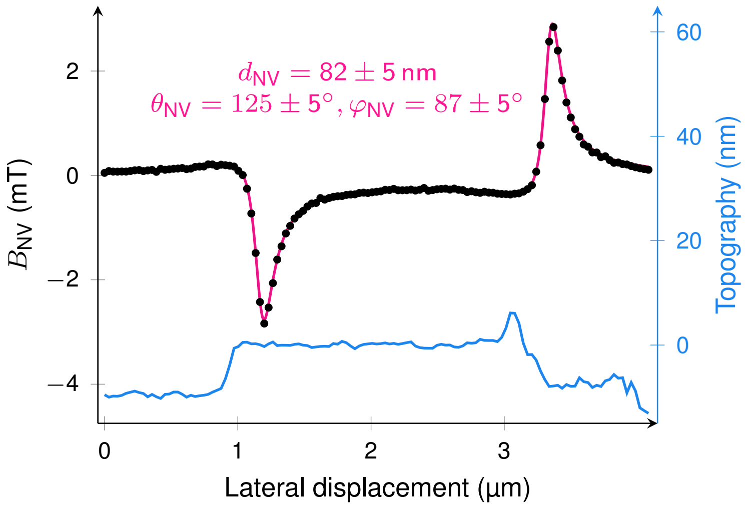


FIG. S2. Calibration experiment of the diamond probe. The measurement is performed on a 2 µm-wide ferromagnetic stripe, with the following composition: $TaN_{0.7\%}$ (1 nm)|$Co_{20}Fe_{60}B_{20}$ (1 nm)|MgO (2 nm) and analyzed following the method detailed in ref. [1]. The indicated value of $d_{NV}$ takes into account the 3 nm-thick Al capping layer.

## III. STRAY FIELD FROM THE EDGE OF A UNIFORMLY MAGNETIZED FILM

We derive here the analytic formula of the stray field present at the edge of an in-plane magnetized layer, which we used to extract the value of $M_s$ in Fig. 2. We consider a semi-infinite film with an edge parallel to the $y$ direction, located at $x = x_0$ and the orientation of the magnetization $\vec{M}$ is decribed by the angles $\theta_M$ and $\varphi_M$, as depicted on the sketch below.

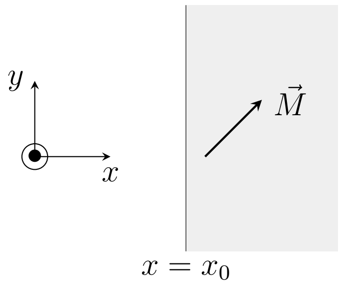


$$\vec{M} = M \begin{pmatrix} \cos\varphi_M \sin\theta_M \\ \sin\varphi_M \sin\theta_M \\ \cos\theta_M \end{pmatrix}$$

We can write the stray field $\vec{B}(\vec{r})$ as

$$\vec{B}(\vec{r}) = \frac{\mu_0}{4\pi} \int_{z'=-\frac{t}{2}}^{\frac{t}{2}} \int_{x'=x_0}^{+\infty} \int_{y'=-\infty}^{+\infty} \left( \frac{3(\vec{r}-\vec{r'})(\vec{M}\cdot(\vec{r}-\vec{r'}))}{|\vec{r}-\vec{r'}|^5} - \frac{\vec{M}}{|\vec{r}-\vec{r'}|^3} \right) \mathrm{d}x'\,\mathrm{d}y'\,\mathrm{d}z' \tag{1}$$

We compute each spatial component separately. Note that as the problem is invariant under a translation along the $y$ axis, $B_y(\vec{r}) = 0$. We start with $B_x$:

$$B_x(\vec{r}) = \frac{\mu_0 M}{4\pi} \int_{z'=-\frac{t}{2}}^{\frac{t}{2}} \int_{x'=x_0}^{+\infty} \int_{y'=-\infty}^{+\infty} \left[ \frac{3(x-x')\left[(x-x')\cos\varphi_M \sin\theta_M + (y-y')\sin\varphi_M \sin\theta_M + (z-z')\cos\theta_M\right]}{\left[(x-x')^2+(y-y')^2+(z-z')^2\right]^{\frac{5}{2}}} - \frac{\cos\varphi_M \sin\theta_M}{\left[(x-x')^2+(y-y')^2+(z-z')^2\right]^{\frac{3}{2}}} \right] \mathrm{d}x'\,\mathrm{d}y'\,\mathrm{d}z'$$

Everything can be integrated analytically, leading to:

$$\boxed{\begin{aligned} B_x(\vec{r}) = -\frac{\mu_0 M}{2\pi} \Bigg[ &\cos\varphi_M \sin\theta_M \left( \arctan\left(\frac{z+\frac{t}{2}}{x-x_0}\right) - \arctan\left(\frac{z-\frac{t}{2}}{x-x_0}\right) \right) \\ &+ \frac{\cos\theta_M}{2} \left( \log\left( \left(z+\frac{t}{2}\right)^2 + (x-x_0)^2 \right) - \log\left( \left(z-\frac{t}{2}\right)^2 + (x-x_0)^2 \right) \right) \Bigg] \end{aligned}} \tag{2}$$

A similar calculation for the component $B_z(\vec{r})$ results in:

$$\boxed{\begin{aligned} B_z(\vec{r}) = \frac{\mu_0 M}{2\pi} \Bigg[ &\cos\theta_M \left( \arctan\left(\frac{z+\frac{t}{2}}{x-x_0}\right) - \arctan\left(\frac{z-\frac{t}{2}}{x-x_0}\right) \right) \\ &- \frac{\cos\varphi_M \sin\theta_M}{2} \left( \log\left( (z+\frac{t}{2})^2 + (x-x_0)^2 \right) - \log\left( (z-\frac{t}{2})^2 + (x-x_0)^2 \right) \right) \Bigg] \end{aligned}} \tag{3}$$

An interesting case is the limit $t \ll z$, meaning that the thickness of the film is much smaller than the distance between the NV center and the sample. Assuming this, we can simplify Eqs 2 and 3 and write:

$$\begin{cases} B_x(\vec{r}) = -\dfrac{\mu_0 M t}{2\pi} \; \dfrac{\cos\varphi_M \sin\theta_M (x - x_0) + \cos\theta_M z}{z^2 + (x - x_0)^2} \\ B_y(\vec{r}) = 0 \\ B_z(\vec{r}) = \dfrac{\mu_0 M t}{2\pi} \; \dfrac{\cos\theta_M (x - x_0) - \cos\varphi_M \sin\theta_M z}{z^2 + (x - x_0)^2} \end{cases} \tag{4}$$

## IV. ESTIMATION OF THE ERROR IN THE EXTRACTION OF $M_s$

We detail here the procedure used to estimate the uncertainty $\varepsilon$ on the estimation of $M_s$, which was previously applied in refs. [2, 3]. The total uncertainty is obtained from the fitting procedure itself and from the uncertainties on the parameters involved. Here these parameters are $d_{\rm NV}$, $t$, $\theta_{\rm NV}$, $\varphi_{\rm NV}$, $\theta_{\rm M}$ and $\varphi_{\rm M}$. Writing all these parameters as $p_i$, we express them as $p_i = \bar{p}_i \pm \sigma_{p_i}$ with $\bar{p}_i$ their nominal value and $\sigma_{p_i}$ their uncertainty. The parameters describing the position and orientation of the NV center are obtained from the independent measurement shown in Fig. S2, the thickness is known from the growth procedure and the orientation of the magnetization is inferred from the images, and thus assumed to be parallel to the $y$ axis. The extracted $M_s$ value is obtained from a fit with the parameters set to their nominal values $\bar{p}_i$.

The uncertainty $\varepsilon_{p_i}$ introduced by each parameter $p_i$ is calculated by performing the fit with $p_i = \bar{p}_i + \sigma_{p_i}$ and $p_i = \bar{p}_i - \sigma_{p_i}$ while all the other parameters $p_j$ are kept at their nominal value $\bar{p}_j$. The resulting values of $M_s$ are denoted as $M_s(\bar{p}_i + \sigma_{p_i})$ and $M_s(\bar{p}_i - \sigma_{p_i})$. Then we compute $\varepsilon_{p_i}$:

$$\varepsilon_{p_i} = \frac{|M_s(\bar{p}_i + \sigma_{p_i}) - M_s| + |M_s(\bar{p}_i - \sigma_{p_i}) - M_s|}{2M_s} \tag{5}$$

Finally, we get the total uncertainty from:

$$\varepsilon = \sqrt{\varepsilon_{\rm fit}^2 + \sum_i \varepsilon_{p_i}^2} \tag{6}$$

since we assume that all the errors are independent. Tables below gather the data for the 4 calculations of $M_s$ shown in Fig. 2. The average value of $M_s$ is $202 \pm 12\,\mathrm{kA\,m^{-1}}$, where we used the standard deviation of the 4 measurements as the uncertainty.

| **Parameter** | **Value** | **Uncertainty** | **Resulting error (%)** |
|---|---|---|---|
| $d_{\rm NV}$ | 119 nm | ± 20 nm | 9% |
| $t$ | 11.8 nm | ± 0.3 nm | 2.5% |
| $\theta_{\rm NV}$ | 125° | ± 5° | 0% |
| $\varphi_{\rm NV}$ | 87° | ± 5° | 0.4% |
| $\theta_{\rm M}$ | 90° | ± 5° | 0% |
| $\varphi_{\rm M}$ | 90° | ± 10° | 1.7% |
| Fit error | | $5.5\,\mathrm{kA\,m^{-1}}$ | 3% |
| | | | Total error: 10% |

TABLE I. Uncertainty estimation for the fit presented in Fig. 2(a), yielding $M_s = 200 \pm 20\,\mathrm{kA\,m^{-1}}$.

| **Parameter** | **Value** | **Uncertainty** | **Resulting error (%)** |
|---|---|---|---|
| $d_{\mathrm{NV}}$ | 96 nm | ± 20 nm | 11% |
| $t$ | 11.8 nm | ± 0.3 nm | 2.5% |
| $\theta_{\mathrm{NV}}$ | 125° | ± 5° | 0.2% |
| $\varphi_{\mathrm{NV}}$ | 87° | ± 5° | 0.4% |
| $\theta_{\mathrm{M}}$ | 90° | ± 5° | 0.3% |
| $\varphi_{\mathrm{M}}$ | 90° | ± 10° | 0.5% |
| Fit error | | 7.5 kA m$^{-1}$ | 4.7% |
| | | | Total error: 12.2% |

TABLE II. Uncertainty estimation for the fit presented in Fig. 2(b), yielding $M_s = 168 \pm 20\,\mathrm{kA\,m^{-1}}$.

| **Parameter** | **Value** | **Uncertainty** | **Resulting error (%)** |
|---|---|---|---|
| $d_{\mathrm{NV}}$ | 127 nm | ± 20 nm | 8.2% |
| $t$ | 11.8 nm | ± 0.3 nm | 2.5% |
| $\theta_{\mathrm{NV}}$ | 125° | ± 5° | 0% |
| $\varphi_{\mathrm{NV}}$ | 87° | ± 5° | 0.3% |
| $\theta_{\mathrm{M}}$ | 90° | ± 5° | 0% |
| $\varphi_{\mathrm{M}}$ | 90° | ± 10° | 0.4% |
| Fit error | | 8.3 kA m$^{-1}$ | 4.3% |
| | | | Total error: 9.6% |

TABLE III. Uncertainty estimation for the fit presented in Fig. 2(c), yielding $M_s = 205 \pm 20\,\mathrm{kA\,m^{-1}}$.

| **Parameter** | **Value** | **Uncertainty** | **Resulting error (%)** |
|---|---|---|---|
| $d_{\mathrm{NV}}$ | 137 nm | ± 20 nm | 7.1% |
| $t$ | 11.8 nm | ± 0.3 nm | 2.5% |
| $\theta_{\mathrm{NV}}$ | 125° | ± 5° | 0% |
| $\varphi_{\mathrm{NV}}$ | 87° | ± 5° | 0.4% |
| $\theta_{\mathrm{M}}$ | 90° | ± 5° | 0.1% |
| $\varphi_{\mathrm{M}}$ | 90° | ± 10° | 0.5% |
| Fit error | | 7.1 kA m$^{-1}$ | 3.2% |
| | | | Total error: 8.2% |

TABLE IV. Uncertainty estimation for the fit presented in Fig. 2(d), yielding $M_s = 234 \pm 19\,\mathrm{kA\,m^{-1}}$.

## V. CHOICE OF $K_u$ IN THE MICROMAGNETIC SIMULATIONS OF THE VORTICES

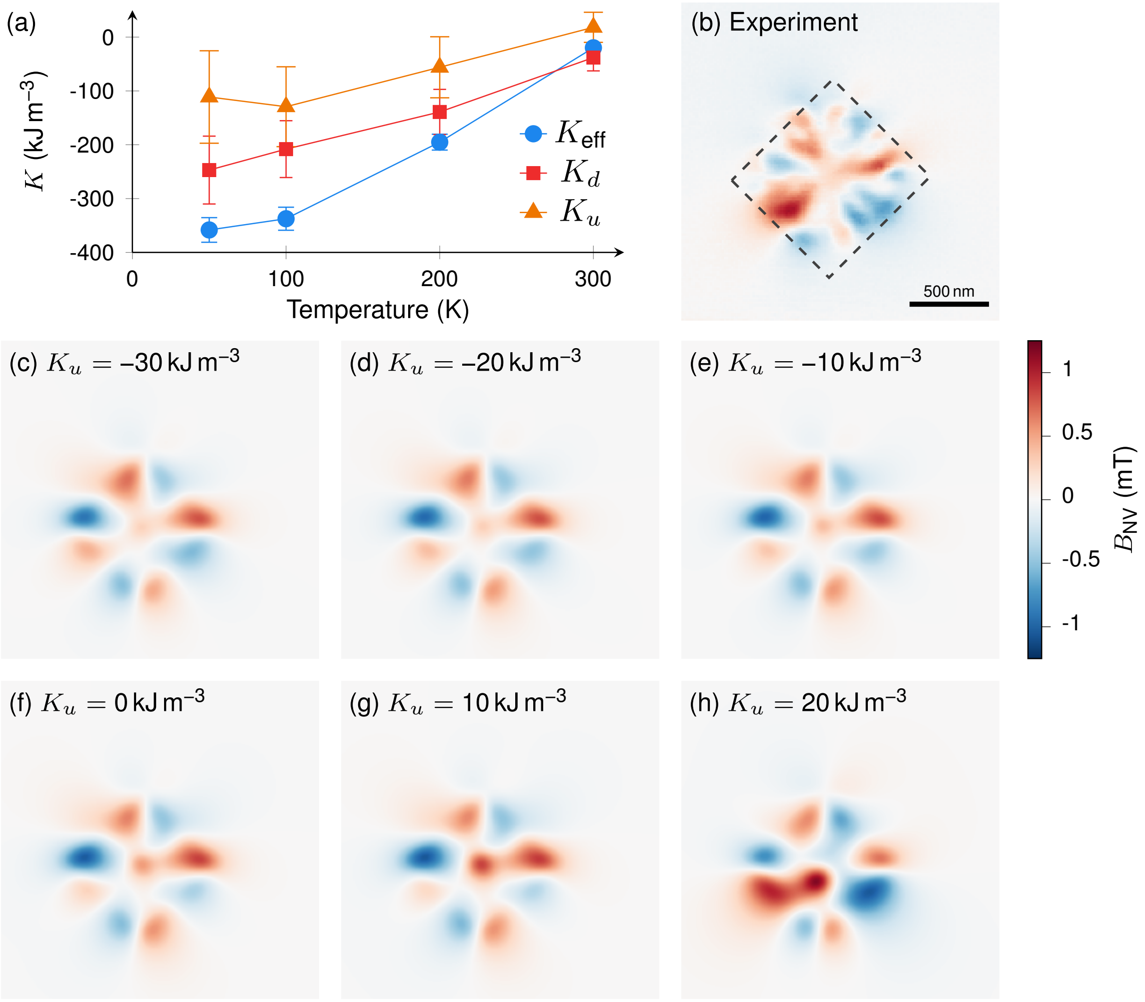


FIG. S3. (a) SQUID measurement of the effective anisotropy $K_{\text{eff}}$, which, combined with the measurement of $M_s$ in Fig. 1 providing the shape anisotropy $K_d$, allows us to obtain the value of the uniaxial anisotropy $K_u$. $K_u$ is very small at room temperature. (b) Measured magnetic stray field map of a vortex in a $1 \times 1\,\mu\text{m}^2$ $Fe_5GeTe_2$ square. (c)-(h) Magnetic stray field maps from vortex configurations obtained with micromagnetic simulations, with the same parameters as specified in the main text except $K_u$, which is varied in the different panels.

## VI. VORTICES IN DISKS

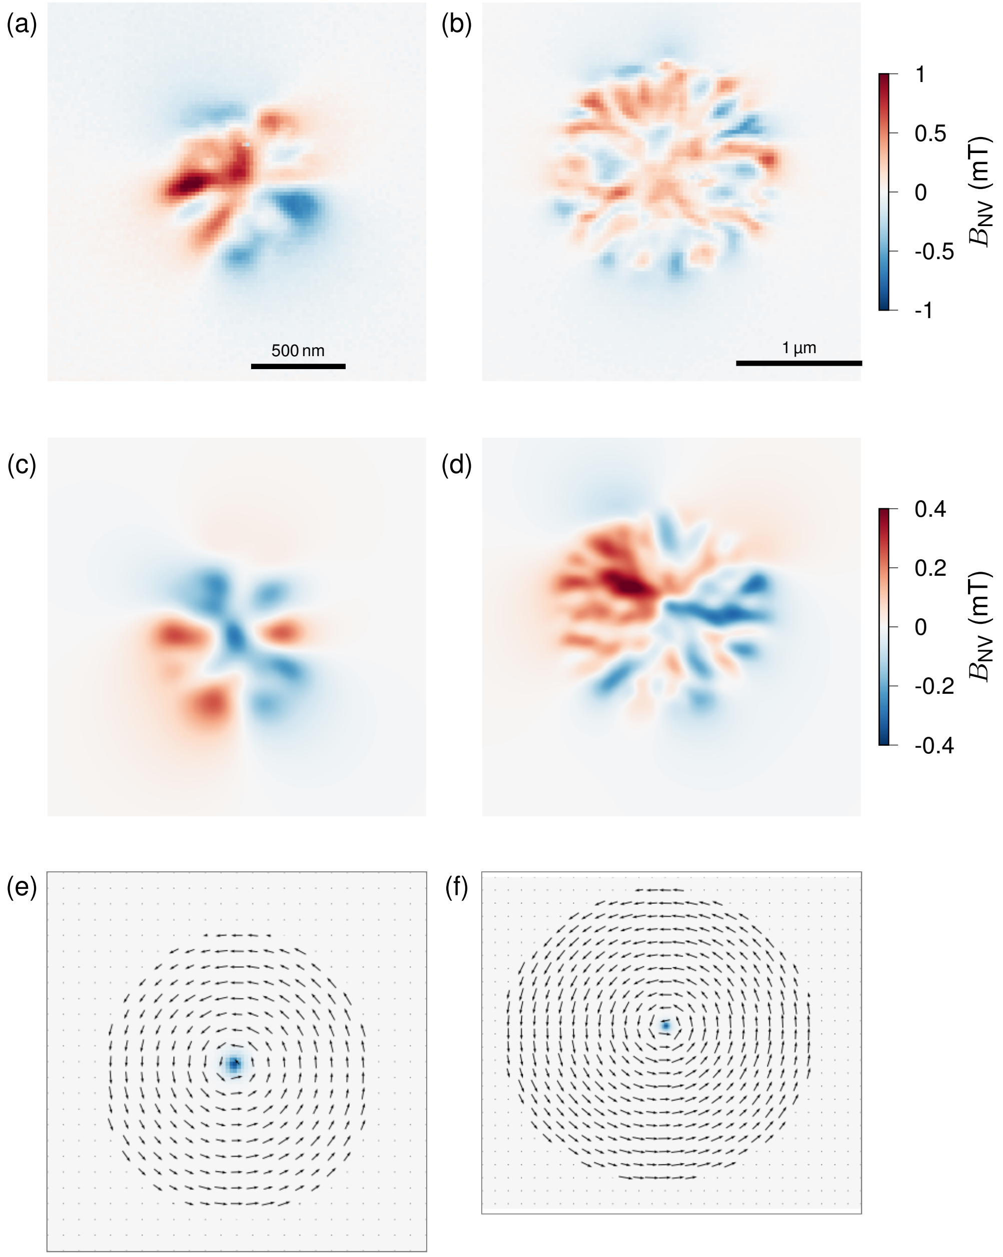


FIG. S4. (a)-(b) Measured stray field maps of vortices in discs microstructures. (c)-(d) Computed stray field maps resulting from the magnetic state shown in (e)-(f). (e)-(f) Magnetization configurations obtained from micromagnetic calculations with the parameters from Table I, with the blue color indicating the core of the vortices where the magnetization tilts out-of-plane. The field strength is significantly lower than in the measurement, probably because $d_{NV}$ was actually smaller than 120 nm during this experiment.

[1] T. Hingant, J.-P. Tetienne, L. J. Martínez, K. Garcia, D. Ravelosona, J.-F. Roch, and V. Jacques, Measuring the Magnetic Moment Density in Patterned Ultrathin Ferromagnets with Submicrometer Resolution, Physical Review Applied **4**, 014003 (2015).

[2] I. Gross, W. Akhtar, V. Garcia, L. J. Martínez, S. Chouaieb, K. Garcia, C. Carrétéro, A. Barthélémy, P. Appel, P. Maletinsky, J.-V. Kim, J. Y. Chauleau, N. Jaouen, M. Viret, M. Bibes, S. Fusil, and V. Jacques, Real-space imaging of non-collinear antiferromagnetic order with a single-spin magnetometer, Nature **549**, 252 (2017).

[3] F. Fabre, A. Finco, A. Purbawati, A. Hadj-Azzem, N. Rougemaille, J. Coraux, I. Philip, and V. Jacques, Characterization of room-temperature in-plane magnetization in thin flakes of $CrTe_2$ with a single-spin magnetometer, Physical Review Materials **5**, 034008 (2021).
